# Supplementary material for: RIDE: Real-time Intrusion Detection via Explainable Machine Learning Implemented in a Memristor Hardware Architecture
Source: arXiv:2311.16018 source file (2023-11-27)
Supplement: Supplementary file 1 [file appendix.tex]

\section*{JSHC Algorithm}
\textcolor{red}{Jingdi: Polish pseudo code for JSHC algorithm, now is a draft}

\begin{algorithm}[H]
\caption{JSHC Algorithm}
\label{alg:JSHC}
\begin{algorithmic}
%\small
   \STATE {\bfseries Input:} X: input data
   \STATE {\bfseries Input:} y: target variable
   \STATE {\bfseries Input:} alpha set: set of ccp alpha parameters
   \STATE {\bfseries Input:} beta set: set of hardware parameters
   \STATE {\bfseries Input:} min beta: minimum value for hardware parameter beta
   \STATE {\bfseries Input:} max beta: maximum value for hardware parameter beta
   \STATE {\bfseries Input:} tol: tolerance for bisection search
   \STATE {\bfseries Input:} max iter: maximum number of iterations for bisection search
   \STATE best alpha = None
   \STATE best beta = None
   \STATE best accuracy = 0
   \STATE {\bfseries Exhaustive search for optimal alpha:}
   \FOR{alpha in alpha set}
      \STATE {\bfseriesGenerate decision tree using current alpha:}
      \STATE tree = generate tree(X, y, alpha)
      \STATE {\bfseriesGenerate Evaluate accuracy for all betas in the set}
      \FOR{beta in beta set}
      \STATE {\bfseriesGenerate Quantize tree using current beta}
      \STATE quantized tree = quantize tree(tree, beta)
      \STATE {\bfseriesGenerate Evaluate accuracy of quantized tree}
      \STATE accuracy = evaluate tree(X, y, quantized tree)
      \STATE {\bfseriesGenerate Update best alpha and beta if current accuracy is higher}
      \IF{accuracy $\ge$ best accuracy}
      \STATE best alpha = alpha
      \STATE best beta = beta
      \STATE best accuracy = accuracy
      \ENDIF
      \ENDFOR
   \ENDFOR
   \STATE Bisection search for optimal beta
   \STATE left = min beta
   \STATE right = max beta
   \WHILE{right - left $\ge$ tol and max iter $\ge$ 0}
      \STATE Calculate mid-point of the range
      \STATE mid = (left + right) / 2
      
      \STATE Generate decision tree using fixed alpha and current beta
      \STATE tree = generate tree(X, y, best alpha)
      \STATE quantized tree = quantize tree(tree, mid)
      
      \STATE Evaluate accuracy of quantized tree
      \STATE accuracy = evaluate tree(X, y, quantized tree)
      
      \STATE Update search range
      \IF{accuracy $\ge$ best accuracy}
         \STATE best beta = mid
         \STATE best accuracy = accuracy
         \STATE left = mid
      \ELSE
         \STATE right = mid
      \ENDIF
      
      \STATE max iter = max iter - 1
   \ENDWHILE
   \STATE {\bfseries Output:} best alpha: optimal ccp alpha parameter
   \STATE {\bfseries Output:} best beta: optimal hardware parameter
   \STATE {\bfseries Output:} best accuracy: classification accuracy achieved by using best alpha and best beta.
   
\end{algorithmic}
\end{algorithm}
